# Supplementary material for: Linear Flows on Translation Prisms
Source: arXiv:2504.08955 ancillary file (2025-04-11)
Supplement: Supplementary file 1 [file appendix_calculations.pdf]

# appendix_calculations

January 15, 2025

## 1 Appendix Calculations

Here we verify the statements made in Appendix A of the paper *Linear flows on translation prisms*.

### 1.1 Prerequisites

This notebook is currently running SageMath 10.4. We also use sage-flatsurf. We are using version 0.5.2.

[1]:
```
import flatsurf
flatsurf.version.version
```

[1]:
```
'0.5.2'
```

The current version, 0.7.1, has errors related to canonicalization. See this bug report. Once this is resolved, I expect the code will run on current versions.

Because we run an old version, we receive several warnings. We disable the printing of these below:

[2]:
```
import warnings
warnings.filterwarnings('ignore', category=DeprecationWarning)
warnings.filterwarnings('ignore', category=UserWarning)
```

### 1.2 Definitions

The appendix makes claims about the following values of $n$:

[3]:
```
n_values = [7, 9, 14, 16, 18, 20, 24, 30]
n_values
```

[3]:
```
[7, 9, 14, 16, 18, 20, 24, 30]
```

The surface $S_n$ can be produced from the following function:

[4]:
```
def S_def(n):
    if n%2 == 1:
        # Odd n
        s = flatsurf.translation_surfaces.veech_double_n_gon(n)
    else:
        # Even n
```

```
        s = flatsurf.translation_surfaces.veech_2n_gon(ZZ(n/2))
    s.set_immutable()
    # Ensure that (1,0) or (-1, 0) is in each polygon.
    for p in s.polygons():
        assert vector([1,0]) in p.edges() or vector([-1,0]) in p.edges()
    # Run flatsurf tests. An error will be raised if this fails.
    TestSuite(s).run()
    return s
```

The number $a_k = 2\cos\frac{\pi}{k}$ is an algebraic real. Note that $k = n$ when $n$ is odd and $k = \frac{n}{2}$ when $n$ is even.

[5]:
```
def a_def(k):
    a_AA = AA(2 * cos(pi/k))
    return a_AA

def k_def(n):
    if n%2 == 1:
        # Odd n
        return n
    else:
        # Even n
        return n/2
```

We use $K$ to denote the number field $\mathbb{Q}(a_k)$. We construct this number field below.

[6]:
```
def K_def(k):
    a_AA = a_def(k)
    K.<a> = NumberField(a_AA.minpoly(), embedding=a_AA)
    return K
```

For each $n$ we defined a matrix $C_n$.

[7]:
```
def C_def(n):
    if n%2 == 1:
        # Odd n
        return matrix(AA, [
            [  1, tan(pi/(2*n)) ],
            [ -1, tan(pi/(2*n)) ]
        ])
    elif n%4 == 0:
        # n divisible by four
        return matrix(AA, [
            [ tan(pi/n), -1 ],
            [         0,  1 ],
        ])
    else:
        # k is odd
        return matrix(AA, [
```

```
            [         0, -sec(pi/n) ],
            [ sin(pi/n), -cos(pi/n) ],
        ])
```

We defined $\omega_n$ to be the surface $C \cdot S_n$. We change the field the surface is defined over to be $K = \mathbb{Q}(a_k)$. We use flatsurf's ability to canonicalize a translation surface to give $\omega_n$ a standard presentation.

[8]:
```
@cached_method
def omega_def(n):
    S = S_def(n).change_ring(AA) # Define over AA so we can multiply by C
    C = C_def(n)
    k = k_def(n)
    K = K_def(k)
    omega = (C*S).change_ring(K).canonicalize()
    # Run flatsurf tests. An error will be raised if this fails.
    TestSuite(omega).run()
    return omega
```

The Veech group elements of $\omega_n$ we use are $A_n$ and $B_n$.

[9]:
```
def A_def(n):
    k = k_def(n)
    K = K_def(k)
    a = K(a_def(k))
    if n%2 == 1:
        # Odd case
        return matrix(K, [
            [1, a],
            [0, 1]
        ])
    else:
        # Even case
        return matrix(K, [
            [1, 2],
            [0, 1]
        ])

def B_def(n):
    k = k_def(n)
    K = K_def(k)
    a = K(a_def(k))
    if n%2 == 1:
        # Odd case
        return matrix(K, [
            [0, -1],
            [1,  0]
        ])
```

```
    else:
        # Even case
        return matrix(K, [
            [      1, 0],
            [1 + a/2, 1]
        ])
```

The matrix $D$ was given both as a matrix and as a word in $\langle A, B \rangle$. Our word will be an element in the free group with generators $A$ and $B$.

```
[10]: def D_word(n):
          free_group.<A,B> = FreeGroup()
          if n == 7:
              return B^-1 * A^-1 * B * A
          if n == 9:
              return B^3 * A^3 * B * A^-4 * (B*A)^2
          if n == 14:
              return A * B^-1 * A^-1 * B
          if n == 16:
              return B^-1 * A * B^-1 * (B^-1 * A)^7 * A^2 * (A^2 * B^-1)^2 * (B^-1 *␣
       ↪A)^5
          if n == 18:
              return B^-3 * A^-1 * B^4 * A * B^-1
          if n == 20:
              return (B^-1 * A)^7 * A^6 * B^-1 * A^4
          if n == 24:
              return (B^-1 * A)^2 * B^-6 * A^-1 * B * A^-5 * B^-1 * A * (B * A^-1)^2␣
       ↪* B^6 * A * B^-1 * A^5 * B * A^-1
          if n == 30:
              return (A * B^-1)^10 * A^17 *B ^-1 * A * (B^-1 * A * B^-1)^2
```

```
[11]: def D_def(n):
          D_free_group_element = D_word(n)
          A = A_def(n)
          B = B_def(n)
          return D_free_group_element(A, B)
```

The dominant eigenvalue of $D_n$ is $\beta_n$. The appendix gives formulas for these in each case. The function `beta_def` will produce these formulas.

```
[12]: def beta_def(n):
          k = k_def(n)
          K = K_def(k)
          a = K(a_def(k))
          if n == 7:
              beta = a^2 + a
          if n == 9:
              beta = 14*a^2 + 26*a + 7
```

```
    if n == 14:
        beta = 4*a^2 + 3*a - 2
    if n == 16:
        beta = 184*a^3 + 340*a^2 - 108*a - 199
    if n == 18:
        beta = 32*a^2 + 60*a + 17
    if n == 20:
        beta = 92*a^3 + 175*a^2 - 127*a - 242
    if n == 24:
        beta = 3916750*a^3 + 7566580*a^2 - 1049490*a - 2027459
    if n == 30:
        beta = 92*a^3 + 272*a^2 + 164*a - 47
    return beta
```

The appendix defines matrices $E_n$ as below.

[13]:
```
def E_def(n):
    k = k_def(n)
    K = K_def(k)
    a = K(a_def(k))
    if n == 7:
        return 1/7 * matrix(K, [
            [ -a^2 - a + 2,     -a^2 - 2*a ],
            [ -a^2 - a + 2, -a^2 + 2*a + 1 ]
        ])
    if n == 9:
        return 1/9 * matrix(K, [
            [ -16*a^2 + 8*a +14, -a^2 - 13*a - 10 ],
            [    2*a^2 + 2*a -4,    2*a^2 - a - 4 ]
        ])
    if n == 14:
        return 1/7 * matrix(K, [
            [     -3*a^2 + 5, 2*a^2 - 2*a - 6 ],
            [ -a^2 - 3*a - 2, 6*a^2 + 2*a - 6 ]
        ])
    if n == 16:
        return 1/4 * matrix(K, [
            [     11*a^3 + 59/2*a^2 + 35/2*a + 1, 7*a^3 + 25*a^2 + 28*a + 11 ],
            [ 23/2*a^3 - 21/2*a^2 - 179/2*a - 57, -6*a^3 - 20*a^2 - 18*a - 3 ]
        ])
    if n == 18:
        return 1/9 * matrix(K, [
            [ -7*a^2 - 7*a + 5,  2*a^2 + 6*a + 4 ],
            [   -4*a^2 - a + 8, 8*a^2 - 4*a - 22 ]
        ])
    if n == 20:
        return 1/5 * matrix(K, [
```

```
            [ 1/2*a^3 + 1/2*a^2 - 2*a - 5/2,         -2*a^3 - a^2 + 5*a ],
            [ 49/2*a^3 + 49*a^2 - 27*a - 60, 8*a^3 + 34*a^2 + 39*a + 10 ]
        ])
    if n == 24:
        return 1/6 * matrix(K, [
            [     -1/2*a^3 - 3/2*a^2 - 1/2*a + 3/2,       2*a^3 + 2*a^2 - 4*a -␣
↪1 ],
            [ 115/2*a^3 + 3/2*a^2 - 383/2*a + 75/2, -44*a^3 + 15*a^2 + 187*a -␣
↪27 ]
        ])
    if n == 30:
        return 1/15 * matrix(K, [
            [ -5*a^3 + 9*a^2 + 49*a + 32,     2*a^3 - 8*a^2 - 32*a - 12 ],
            [ 23*a^3 + 82*a^2 + 76*a + 9, -14*a^3 - 70*a^2 - 100*a - 36 ]
        ])
```

## 1.3 Proofs

### 1.3.1 Ring of integers claims

In the start of sections A.1 and A.2, we assert that the ring of integers in $K = \mathbb{Q}(a_n)$ is $\mathbb{Z}[a_k]$. As the ring of integers in a number field is also the maximal order in the number field, we can check this statement as below.

[14]:
```
for n in n_values:
    k = k_def(n)
    K = K_def(k)
    a = K(a_def(k)) # Convert a into the field K.
    if ZZ[a].is_maximal():
        print(f'n={n}: Z[a_{k}] is maximal.')
    else:
        print(f'ERROR: n={n}: Z[a_{k}] is not maximal.')
```

```
n=7: Z[a_7] is maximal.
n=9: Z[a_9] is maximal.
n=14: Z[a_7] is maximal.
n=16: Z[a_8] is maximal.
n=18: Z[a_9] is maximal.
n=20: Z[a_10] is maximal.
n=24: Z[a_12] is maximal.
n=30: Z[a_15] is maximal.
```

### 1.3.2 Claims about polygons making up $\omega_n$.

We need to be able to test if a polygon is a rectangle.

[15]:
```
def is_rectangle(polygon):
    if len(polygon.edges()) != 4:
        # Not a quadrilateral
```

```
        return False
    # We check that each edge is horizontal if and only if the next is vertical.
    for i in range(4):
        if not ((polygon.edge(i)[1] == 0) == (polygon.edge(i+1)[0] == 0)):
            return False
    return True
```

We need to be able to check if a rectangle is a $1 \times 1$ square.

[16]:
```
def is_unit_square(polygon):
    if len(polygon.edges()) != 4:
        # Not a quadrilateral
        return False
    for v in [ vector([0,0]), vector([1,0]), vector([1,1]), vector([0,1]) ]:
        if not v in polygon.vertices():
            return False
    return True
```

We need to be able to find the collection of polygons of largest area in a translation surface.

[17]:
```
def largest_area_polygons(translation_surface):
    all_polygons = list(translation_surface.polygons())
    largest_polygons = [all_polygons[0],]
    largest_area = all_polygons[0].area()
    for polygon in all_polygons[1:]: # Iterate over polygons, skipping the first
        if polygon.area() >= largest_area:
            if polygon.area() == largest_area:
                # Tied for longest. Add to the list of longest
                largest_polygons.append(polygon)
            else:
                # This is larger than the previous largest.
                largest_polygons = [polygon,]
                largest_area = polygon.area()
    return largest_polygons
```

In A.1, we claim that when $n$ is odd, the surface $\omega_n$ is built from $n-2$ rectangles and whose largest area polygon is a unit square.

[18]:
```
for n in n_values:
    if n%2 == 1: # Only consider odd case.
        errors = False
        omega = omega_def(n)
        if len(omega.polygons()) != n-2:
            errors=True
            print(f'ERROR: n={n}: There are not n-2 polygons making up␣
↪omega_{n}.')
        for polygon in omega.polygons():
            if not is_rectangle(polygon):
```

```
                errors=True
                print(f'ERROR: n={n}: One polygon is not a rectangle.')
        largest_polygons = largest_area_polygons(omega)
        if len(largest_polygons) != 1:
            errors=True
            print(f'ERROR: n={n}: There is not a unique polygon of largest area.
 ↪')
        if not is_unit_square(largest_polygons[0]):
            errors=True
            print(f'ERROR: n={n}: The largest polygon is not a unit square.')
        if not errors:
            print(f'n={n}: All checks were passed.')
```

```
n=7: All checks were passed.
n=9: All checks were passed.
```

In A.2, we claim that when $n$ is even, the surface is defined over $\mathbb{Q}(a_k)$, the surface is decomposed into rectangles, and that the largest rectangle is again a unit square. Here we check this.

[19]:
```
for n in n_values:
    if n%2 == 0: # Only consider even case.
        errors = False
        omega = omega_def(n)
        k = k_def(n)
        K = K_def(k)
        if omega.base_ring() != K:
            errors=True
            print(f'ERROR: n={n}: The surface omega_{n} is not defined over␣
 ↪K_{k}.')
        for polygon in omega.polygons():
            if not is_rectangle(polygon):
                errors=True
                print(f'ERROR: n={n}: One polygon is not a rectangle.')
        largest_polygons = largest_area_polygons(omega)
        if len(largest_polygons) != 1:
            errors=True
            print(f'ERROR: n={n}: There is not a unique polygon of largest area.
 ↪')
        if not is_unit_square(largest_polygons[0]):
            errors=True
            print(f'ERROR: n={n}: The largest polygon is not a unit square.')
        if not errors:
            print(f'n={n}: All checks were passed.')
```

```
n=14: All checks were passed.
n=16: All checks were passed.
n=18: All checks were passed.
n=20: All checks were passed.
```

```
n=24: All checks were passed.
n=30: All checks were passed.
```

### 1.3.3 The Veech groups

We claim that the matrices $A_n$ and $B_n$ lie in the Veech groups of $\omega_n$. To check that a matrix $M$ is in the Veech group of a surface $s$, we check that the canonicalizations of $M \cdot s$ and $s$ are equal.

[20]:
```
for n in n_values:
    errors = False
    omega = omega_def(n)
    A = A_def(n)
    if (A*omega).canonicalize() != omega.canonicalize():
        errors=True
        print(f'ERROR: n={n}: The matrix A_{n}={A} is not in the Veech group of␣
↪omega_{n}.')
    B = B_def(n)
    if (B*omega).canonicalize() != omega.canonicalize():
        errors=True
        print(f'ERROR: n={n}: The matrix B_{n}={B} is not in the Veech group of␣
↪omega_{n}.')
    if not errors:
        print(f'n={n}: Both A_{n} and B_{n} lie in the Veech group of omega_{n}.
↪')
```

```
n=7: Both A_7 and B_7 lie in the Veech group of omega_7.
n=9: Both A_9 and B_9 lie in the Veech group of omega_9.
n=14: Both A_14 and B_14 lie in the Veech group of omega_14.
n=16: Both A_16 and B_16 lie in the Veech group of omega_16.
n=18: Both A_18 and B_18 lie in the Veech group of omega_18.
n=20: Both A_20 and B_20 lie in the Veech group of omega_20.
n=24: Both A_24 and B_24 lie in the Veech group of omega_24.
n=30: Both A_30 and B_30 lie in the Veech group of omega_30.
```

### 1.3.4 The matrices $D_n$

The method `D_words` defined above defines $D_n$ as a word in our chosen Veech group generators $A_n$ and $B_n$. This word was converted to a matrix in `D_def`. The appendix provides matrix versions of $D_n$. We print out the values of the matrices $D$ produced by `D_def` below. It may be observed that the matrices here match the ones in the appendix.

[21]:
```
for n in n_values:
    D = D_def(n)
    print(f'The matrix D_{n} is')
    show(D)
```

```
The matrix D_7 is
```

$$\begin{pmatrix} 1 & a \\ a & a^2+1 \end{pmatrix}$$

The matrix D_9 is

$$\begin{pmatrix} -4a^2 - 1 & -9a - 4 \\ 40a + 12 & 28a^2 + 12a - 1 \end{pmatrix}$$

The matrix D_14 is

$$\begin{pmatrix} a^2 + 3a + 3 & 2a + 4 \\ \frac{1}{2}a^2 + 2a + 2 & a + 3 \end{pmatrix}$$

The matrix D_16 is

$$\begin{pmatrix} -900a^3 - 1547a^2 + 831a + 1141 & -772a^3 - 1406a^2 + 516a + 890 \\ 1112a^3 + \frac{3939}{2}a^2 - 874a - 1324 & 996a^3 + 1819a^2 - 639a - 1107 \end{pmatrix}$$

The matrix D_18 is

$$\begin{pmatrix} 4a^2 + 12a + 9 & -8a - 16 \\ -32a^2 - 74a - 38 & 12a^2 + 52a + 57 \end{pmatrix}$$

The matrix D_20 is

$$\begin{pmatrix} -18a^3 - 31a^2 + 29a + 43 & -132a^3 - 234a^2 + 208a + 330 \\ 12a^3 + \frac{49}{2}a^2 - 11a - 27 & 90a^3 + 183a^2 - 83a - 203 \end{pmatrix}$$

The matrix D_24 is

$$\begin{pmatrix} 1384810a^3 + 2678580a^2 - 362410a - 712559 & -2102180a^3 - 4065520a^2 + 552020a + 1082920 \\ -1667820a^3 - 3220180a^2 + 450780a + 864120 & 2530790a^3 + 4887020a^2 - 682790a - 1311239 \end{pmatrix}$$

The matrix D_30 is

$$\begin{pmatrix} 401a^3 + 1187a^2 + 706a - 223 & -288a^3 - 866a^2 - 516a + 190 \\ \frac{867}{2}a^3 + 1268a^2 + 730a - \frac{513}{2} & -321a^3 - 931a^2 - 498a + 241 \end{pmatrix}$$

### 1.3.5 The eigenvalues of $D_n$

Here we check that the eigenvalues of $D_n$ are given by

$$\left\{\beta_n, \frac{1}{\beta_n}\right\}.$$

[22]:
```
for n in n_values:
    D = D_def(n)
    beta = beta_def(n)
    if set(D.eigenvalues()) == {beta, 1/beta}:
        print(f'When n={n}, the eigenvalues of D_{n} are as claimed.')
    else:
        print(f'ERROR: When n={n}, the eigenvalues of D_{n} are DIFFERENT THAN␣
 ↪claimed.')
```

```
When n=7, the eigenvalues of D_7 are as claimed.
When n=9, the eigenvalues of D_9 are as claimed.
When n=14, the eigenvalues of D_14 are as claimed.
```

```
When n=16, the eigenvalues of D_16 are as claimed.
When n=18, the eigenvalues of D_18 are as claimed.
When n=20, the eigenvalues of D_20 are as claimed.
When n=24, the eigenvalues of D_24 are as claimed.
When n=30, the eigenvalues of D_30 are as claimed.
```

Now we check that the eigenvalues are Pisot. We use the following function to check if a number is Pisot.

[23]:
```
def is_pisot(algebraic_number):
    if abs(algebraic_number) <= 1:
        return False
    # Convert the number into the field of algebraic complex numbers
    algebraic_number_QQbar = QQbar(algebraic_number)
    # Construct the algebraic conjugates:
    conjugates = set(algebraic_number_QQbar.minpoly().roots(QQbar,␣
 ↪multiplicities=False)) \
        .difference({algebraic_number_QQbar,})
    # Check that each has absolute value less than one:
    for conj in conjugates:
        if abs(conj) >= 1:
            return False
    return True
```

We check that the expanding eigenvalue $\beta_n$ of $D_n$ is Pisot in all cases:

[24]:
```
for n in n_values:
    beta = beta_def(n)
    if is_pisot(beta):
        print(f'n={n}: The number beta_{n} is Pisot.')
    else:
        print(f'ERROR: n={n}: The number beta_{n} is NOT Pisot.')
```

```
n=7: The number beta_7 is Pisot.
n=9: The number beta_9 is Pisot.
n=14: The number beta_14 is Pisot.
n=16: The number beta_16 is Pisot.
n=18: The number beta_18 is Pisot.
n=20: The number beta_20 is Pisot.
n=24: The number beta_24 is Pisot.
n=30: The number beta_30 is Pisot.
```

Finally, we print out $\beta_n$ with its decimal approximation.

[25]:
```
for n in n_values:
    beta = beta_def(n)
    print(f'beta_{n} = {beta} is approximately {beta.n():0.4f}.')
```

```
beta_7 = a^2 + a is approximately 5.0489.
beta_9 = 14*a^2 + 26*a + 7 is approximately 105.3133.
```

```
beta_14 = 4*a^2 + 3*a - 2 is approximately 16.3937.
beta_16 = 184*a^3 + 340*a^2 - 108*a - 199 is approximately 1923.0651.
beta_18 = 32*a^2 + 60*a + 17 is approximately 242.7900.
beta_20 = 92*a^3 + 175*a^2 - 127*a - 242 is approximately 782.7233.
beta_24 = 3916750*a^3 + 7566580*a^2 - 1049490*a - 2027459 is approximately
52422803.8598.
beta_30 = 92*a^3 + 272*a^2 + 164*a - 47 is approximately 2003.5977.
```

### 1.3.6 The $E_n$ matrices

We claimed that for each $n$ under consideration, we have

$$E_n \cdot D_n \cdot E_n^{-1} = \begin{pmatrix} \beta_n & 0 \\ 0 & 1/\beta_n \end{pmatrix}.$$

Here we check this.

[26]:
```
for n in n_values:
    D = D_def(n)
    E = E_def(n)
    beta = beta_def(n)
    diag = diagonal_matrix([beta, 1/beta])
    if E*D*E^-1 == diag:
        print(f'n={n}: The conjugacy equation holds.')
    else:
        print(f'ERROR: n={n}: The conjugacy equation DOES NOT hold.')
```

```
n=7: The conjugacy equation holds.
n=9: The conjugacy equation holds.
n=14: The conjugacy equation holds.
n=16: The conjugacy equation holds.
n=18: The conjugacy equation holds.
n=20: The conjugacy equation holds.
n=24: The conjugacy equation holds.
n=30: The conjugacy equation holds.
```

### 1.3.7 The eigenvalues

The appendix claims that for the surface $E \cdot \omega_n$, the eigenvalues for both the horizontal and vertical flows are given by the ring of integers $\mathbb{Z}[a]$.

The surface $E \cdot \omega_n$ is invariant under a pseudo-Anosov $\rho_E$ with diagonal derivative, obtained by pushing forward the pseudo Anosov on $\omega_n$. According to Theorem 3.1, the eigenvalues in the horizontal and vertical directions are given by $\mathrm{FA}(\rho_E)$ and $\mathrm{FA}(\rho_E^{-1})$ respectively. To compute this, we use ideas from section 3.1 of the paper.

**Computing $\eta^u$ and $\eta^s$** The cohomology classes $\eta^u, \eta^s \in H^1(E \cdot \omega_n; \mathbb{R})$ measure holonomy in the horizontal and vertical directions respectively. We choose a generating set for $\gamma_1, \ldots, \gamma_m \in H_1(E \cdot \omega_n; \mathbb{Z})$ and represent $\eta^u$ and $\eta^v$ as vectors whose $i$-th entry is $\eta^u(\gamma_i)$ and $\eta^s(\gamma_i)$, respectively.

It seems simplest to choose a generating set for homology on the surface $S_n$ and push it forward to to $E \cdot \omega_n$. First observe the following about each surface:

[27]:
```
for n in n_values:
    S = S_def(n)
    print(f'The surface S_{n} has genus {S.genus()} and {S.num_singularities()}␣
↪singularities.')
```

```
The surface S_7 has genus 3 and 1 singularities.
The surface S_9 has genus 4 and 1 singularities.
The surface S_14 has genus 3 and 2 singularities.
The surface S_16 has genus 4 and 1 singularities.
The surface S_18 has genus 4 and 2 singularities.
The surface S_20 has genus 5 and 1 singularities.
The surface S_24 has genus 6 and 1 singularities.
The surface S_30 has genus 7 and 2 singularities.
```

We observe that $S_n$ has one singularity unless $n \equiv 2 \pmod 4$, in which case it has two singularities. For cases with one singularity, we can use the edges of the first polygon (with label 0) as a generating set for $H_1(S_n; \mathbb{Z})$. When $n \equiv 2 \pmod 4$, observe that the singularities alternate as we move around the single polygon. Vertices of a polygon in the program are numbered cyclically, and we choose for our basis the diagonals connecting vertex $v_j$ to vertex $v_{j+2}$ when $j$ is even.

We care about the holonomy of these classes in $S_n$. The holonomy of the $i$-th generator of $H_1(S_n; \mathbb{Z})$ will appear as the $i$-th column of the following matrix returned by `holonomy_S`.

[28]:
```
def holonomy_S(n):
    S = S_def(n)
    if n%4 == 2:
        return matrix(AA, [S.polygon(0).vertex(j+2) - S.polygon(0).vertex(j)␣
↪for j in range(n)]).transpose()
    else:
        return matrix(AA, [S.polygon(0).edge(i) for i in range(n)]).transpose()

for n in n_values:
    print(f'The holonomy matrix for S_{n} is')
    show(holonomy_S(n))
```

```
The holonomy matrix for S_7 is
```

$$\begin{pmatrix} 1 & 0.6234898018587335? & -0.2225209339563144? & -0.9009688679024191? & -0.9009688679024191? & -0.22252 \\ 0 & 0.7818314824680299? & 0.9749279121818236? & 0.4338837391175581? & -0.4338837391175581? & -0.97492 \end{pmatrix}$$

```
The holonomy matrix for S_9 is
```

$$\begin{pmatrix} 1 & 0.7660444431189781? & 0.1736481776669304? & -\frac{1}{2} & -0.9396926207859084? & -0.939692620 \\ 0 & 0.6427876096865393? & 0.9848077530122081? & 0.866025403784439? & 0.3420201433256688? & -0.342020143 \end{pmatrix}$$

```
The holonomy matrix for S_14 is
```

$$\begin{pmatrix} 1.900968867902420? & 1.524458669761153? & 0.8460107358150480? & 0 & -0.84601073581504 \\ 0.4338837391175582? & 1.215715221585588? & 1.756759394649854? & 1.949855824363648? & 1.7567593946498 \end{pmatrix}$$

```
The holonomy matrix for S_16 is
```

$$\left(\begin{matrix} 1 & 0.9238795325112868? & 0.7071067811865475? & 0.3826834323650898? & 0 & -0.3826834323650898? & -0.70710 \\ 0 & 0.3826834323650898? & 0.7071067811865475? & 0.9238795325112868? & 1 & 0.9238795325112868? & 0.70710 \end{matrix}\right.$$

```
The holonomy matrix for S_18 is
```

$$\left(\begin{matrix} 1.939692620785909? & 1.705737063904887? & 1.266044443118978? & 0.6736481776669304? & \\ 0.3420201433256688? & 0.9848077530122081? & 1.508813013470978? & 1.850833156796647? & 1.969615506024417 \end{matrix}\right.$$

```
The holonomy matrix for S_20 is
```

$$\left(\begin{matrix} 1 & 0.9510565162951536? & 0.8090169943749474? & 0.5877852522924731? & 0.3090169943749474? & 0 & -0.3090169 \\ 0 & 0.3090169943749474? & 0.5877852522924731? & 0.8090169943749474? & 0.9510565162951536? & 1 & 0.951056 \end{matrix}\right.$$

```
The holonomy matrix for S_24 is
```

$$\left(\begin{matrix} 1 & 0.9659258262890683? & 0.866025403784439? & 0.7071067811865475? & \frac{1}{2} & 0.2588190451025 \\ 0 & 0.2588190451025208? & \frac{1}{2} & 0.7071067811865475? & 0.866025403784439? & 0.9659258262890 \end{matrix}\right.$$

```
The holonomy matrix for S_30 is
```

$$\left(\begin{matrix} 1.978147600733806? & 1.891693058376407? & 1.722562452017549? & 1.478147600733806? & 1.169130606358859 \\ 0.2079116908177594? & 0.6146483338935595? & 0.994521895368274? & 1.330930077769868? & 1.609170229261833 \end{matrix}\right.$$

We have $E \cdot \omega_n = E \cdot C \cdot S_n$, so we can compute the horizontal holonomy vector $\eta^u$ on $E \cdot \omega_n$ and the vertical holonomy vector $\eta^s$ on $E \cdot \omega_n$ by

$$\eta^u = (E \cdot C \cdot M)_1 \quad \text{and} \quad \eta^s = (E \cdot C \cdot M)_2$$

where $M$ is the matrix returned by `holonomy_S(n)` and the subscripts of 1 and 2 denote the choice of row vector. We ensure that the returned vector is defined over the trace field $K = \mathbb{Q}(a)$.

The following two functions return $\eta^u$ and $\eta^s$, respectively.

[29]:
```
def eta_u_def(n):
    k = k_def(n)
    K = K_def(k)
    C = C_def(n)
    E = E_def(n)
    return vector(K, (E*C*holonomy_S(n)).row(0))

def eta_s_def(n):
    k = k_def(n)
    K = K_def(k)
    C = C_def(n)
    E = E_def(n)
    return vector(K, (E*C*holonomy_S(n)).row(1))
```

The following function `eta_def(subscript, n)` either returns $\eta^u$ or $\eta^s$ depending if `subscript=='u'` or `subscript=='s'`, respectively.

[30]:
```
def eta_def(subscript, n):
    if subscript == 'u':
```

```
        return eta_u_def(n)
    elif subscript == 's':
        return eta_s_def(n)
    raise ValueError('Invalid subscript')
```

**The ring of integers is contained in FA** Loosely following the paper, we let $\mathrm{FA} \subset \mathbb{R}$ denotes the collection of real numbers $c \in \mathbb{R}$ such that $c\eta$ is forward asymptotic to an integer class (class in $H^1(E \cdot \omega; \mathbb{Z})$) under powers of $\rho^*$ in the unstable case and under powers of $(\rho^{-1})^*$ in the stable case.

Here we will check that the ring of integers $\mathbb{Z}[a]$ is contained in FA.

Observe that if $c \in \mathbb{Z}[a]$, then $c\eta$ is defined over $K$. Let $\sigma$ denote $\rho$ in the unstable case, and denote $\rho^{-1}$ in the stable case. Then $\sigma^n(c\eta) = \beta^n c\eta$. Then if aut is an automorphism of $K$, we have

$$\sigma^n(\mathrm{aut}(c\eta)) = \mathrm{aut}(\beta^n)\mathrm{aut}(c\eta).$$

Since $\beta$ is Pisot, for any nontrivial automorphism, we have $\mathrm{aut}(\beta^n) \to 0$ as $n \to +\infty$. Thus, $c\eta$ is forward asymptotic to the sum of $\mathrm{aut}(c\eta)$ over automorphisms of $K$. So, to show $\mathbb{Z}[a] \subset FA$, it suffices to show that the sum of $\mathrm{aut}(c\eta)$ over the automorphisms is an integer class.

In order to carry this out, we define two functions that make it easier.

The collection of automorphisms of the field $K = \mathbb{Q}(a)$ is available from `K.automorphisms()`. Given such an automorphism `aut` and a vector `v` with entries in $K$, the following function `automorphism_applied_to_vector(aut, v)` applies the automorphisms `aut` to all entries in `v` and returns the result.

The function `sum_over_automorphisms` below takes as input the field $K$ and a $v$ vector with entries in $K$, and returns the sum of automorphisms of $K$ applied to $v$. Because $K$ is Galois, this sum will always be a rational vector.

[31]:
```
def automorphism_applied_to_vector(aut, v):
    return vector([aut(entry) for entry in v])

def sum_over_automorphisms(K, v):
    return sum([automorphism_applied_to_vector(aut, v) for aut in K.
 ↪automorphisms()])
```

The following function returns `True` if we can show by the above method that $\mathbb{Z}[a]$ is contained in FA and returns `False` otherwise. Since both are abelian groups, it suffices to check that a generating set of $\mathbb{Z}[a]$ is contained in FA. We check using the generating set $1, a, a^2, \ldots, a^{d-1}$ where $d$ is the degree of $K$.

[32]:
```
def check_containment_in_FA(subscript, n):
    eta = eta_def(subscript, n)
    k = k_def(n)
    K = K_def(k)
    a = a_def(k)
    for i in range(K.degree()):
        if not sum_over_automorphisms(K, a^i*eta) in ZZ^(eta.degree()):
```

```
            return False
    return True
```

We now check that the ring of integers $\mathbb{Z}[a]$ is contained in F$A$ for each $n$ in the appendix in both the unstable and stable cases:

[33]:
```
for n in n_values:
    for subscript in ['u', 's']:
        if subscript == 'u':
            pseudo_anosov = 'rho'
        else:
            pseudo_anosov = 'rho^-1'
        if check_containment_in_FA(subscript, n):
            print(f'{n}{subscript}: The ring of integers is contained in␣
 ↪FA({pseudo_anosov}).')
        else:
            print(f'ERROR {n}{subscript}: The ring of integers is NOT contained␣
 ↪in FA({pseudo_anosov}).')
```

```
7u: The ring of integers is contained in FA(rho).
7s: The ring of integers is contained in FA(rho^-1).
9u: The ring of integers is contained in FA(rho).
9s: The ring of integers is contained in FA(rho^-1).
14u: The ring of integers is contained in FA(rho).
14s: The ring of integers is contained in FA(rho^-1).
16u: The ring of integers is contained in FA(rho).
16s: The ring of integers is contained in FA(rho^-1).
18u: The ring of integers is contained in FA(rho).
18s: The ring of integers is contained in FA(rho^-1).
20u: The ring of integers is contained in FA(rho).
20s: The ring of integers is contained in FA(rho^-1).
24u: The ring of integers is contained in FA(rho).
24s: The ring of integers is contained in FA(rho^-1).
30u: The ring of integers is contained in FA(rho).
30s: The ring of integers is contained in FA(rho^-1).
```

**Checking that FA equals the ring of integers** In section 3.1, the vector space $V$ is the span of $\eta$ and its algebraic conjugates. Since $K$ is a Galois extension (checked in the function), the algebraic conjugates are all in $K$. Thus, $V$ is defined over $K$. Similar to $\eta$, an element $v \in V$ is taken to be a vector whose $i$-th entry is $v(\gamma_i)$, where $\gamma_i$ is again the $i$-th element of our generating set for $H_1(E \cdot \omega_n; \mathbb{Z})$. We return this version of $V$ in the function `V_def` below:

[34]:
```
def V_def(superscript, n):
    k = k_def(n)
    K = K_def(k)
    # We check that K is Galois below. If it is not Galois, an assertion error␣
 ↪will be raised.
    assert K.is_galois(), f'ERROR n={n}: The field K is not Galois.'
```

```
    eta = eta_def(superscript, n)
    VS = VectorSpace(QQbar, len(eta))
    conjugates = []
    for aut in K.automorphisms():
        # Add to the list of conjugates, the vector formed by applying
        # the automorphism aut to each entry of eta.
        conjugates.append(automorphism_applied_to_vector(aut, eta))
    return VS.span(conjugates)
```

Also from section 3.1, $V_{\mathbb{Z}}$ is $V \cap H^1(E \cdot \omega; \mathbb{Z})$. The function `V_ZZ_def` returns $V_{\mathbb{Z}}$:

[35]:
```
def V_ZZ_def(superscript, n):
    V = V_def(superscript, n)
    return V.change_ring(ZZ).intersection(ZZ^V.degree())
```

As shown in the proof of Proposition 3.2, the set of integer classes to which elements of $L = \{c\eta : \ c \in \mathbb{R}\}$ are forward asymptotic to is $V_{\mathbb{Z}}$. Furthermore, this map $\{c\eta : \ c \in \mathrm{FA}\} \to V_{\mathbb{Z}}$ is a bijection. We have already shown that $\mathbb{Z}[a] \subset \mathrm{FA}$. To show equality, we can show that the image of $\mathbb{Z}[a]$ under the map is equal to $V_{\mathbb{Z}}$.

From the previous part, we know that for each $c \in \mathbb{Z}[a]$, the integer class that $c\eta$ is asymptotic to is the sum over the automorphisms of $K$ of $\mathrm{aut}(c\eta)$.

This check is carried out by the following function which returns `True` if $\mathbb{Z}[a] = \mathrm{FA}$ and `False` otherwise.

[36]:
```
def check_equals_FA(superscript, n):
    V_ZZ = V_ZZ_def(superscript, n)
    eta = eta_def(superscript, n)
    k = k_def(n)
    K = K_def(k)
    a = a_def(k)
    asymototic_integer_vectors = []
    for i in range(K.degree()):
        asymototic_integer_vectors.append(
            V_ZZ.ambient_module()(sum_over_automorphisms(K, a^i*eta))
        )
    image_of_ring_of_integers = V_ZZ.ambient_module().
 ↪span(asymototic_integer_vectors)
    return image_of_ring_of_integers == V_ZZ
```

We now call the function above repeatedly to check that the ring of integers $\mathbb{Z}[a]$ is equal to $FA$ for each $n$ in the appendix in both the unstable and stable cases:

[37]:
```
for n in n_values:
    for superscript in ['u', 's']:
        if subscript == 'u':
            pseudo_anosov = 'rho'
        else:
```

```
            pseudo_anosov = 'rho^-1'
        if check_equals_FA(subscript, n):
            print(f'{n}{subscript}: The ring of integers equals␣
↪FA({pseudo_anosov}).')
        else:
            print(f'ERROR {n}{subscript}: The ring of integers is NOT equal to␣
↪FA({pseudo_anosov}).')
```

```
7s: The ring of integers equals FA(rho^-1).
7s: The ring of integers equals FA(rho^-1).
9s: The ring of integers equals FA(rho^-1).
9s: The ring of integers equals FA(rho^-1).
14s: The ring of integers equals FA(rho^-1).
14s: The ring of integers equals FA(rho^-1).
16s: The ring of integers equals FA(rho^-1).
16s: The ring of integers equals FA(rho^-1).
18s: The ring of integers equals FA(rho^-1).
18s: The ring of integers equals FA(rho^-1).
20s: The ring of integers equals FA(rho^-1).
20s: The ring of integers equals FA(rho^-1).
24s: The ring of integers equals FA(rho^-1).
24s: The ring of integers equals FA(rho^-1).
30s: The ring of integers equals FA(rho^-1).
30s: The ring of integers equals FA(rho^-1).
```

### 1.4 Cohomology class of an eigenfunction

In Appendix C, we need to know the cohomology class of the eigenfunction $\Psi_c : S_7 \to \mathbb{R}/\mathbb{Z}$ where

$$c = \frac{1}{\left\| C_7^{-1} E_7^{-1} \left( \begin{smallmatrix} 0 \\ 1 \end{smallmatrix} \right) \right\|}.$$

This function is obtained by pulling back the eigenfunction for the flow in the vertical direction with eigenvalue 1 on $E \cdot \omega_7$. The cohomology class representing vertical holonomy on $E \cdot \omega_7$ is $\eta_s$, which obtain below:

[38]:
```
eta_s = eta_s_def(7)
show(eta_s)
```

$$\left(-\frac{3}{7}a + \frac{1}{7}, -\frac{1}{7}a^2 - \frac{1}{7}a + \frac{2}{7}, \frac{2}{7}a - \frac{3}{7}, \frac{1}{7}a + \frac{2}{7}, \frac{3}{7}a^2 - \frac{2}{7}a - \frac{2}{7}, -\frac{1}{7}a^2 + \frac{2}{7}a + \frac{1}{7}, -\frac{1}{7}a^2 + \frac{1}{7}a - \frac{1}{7}\right)$$

Here, the entries of `eta_s` represent $\left(\eta_s \circ E_7 \circ C_7(e_i)\right)_{i=0}^{6}$ where $e_i$ is an edge of the heptagon with label 0 oriented counterclockwise, and we abuse notation by using $E_7 \circ C_7$ to denote the affine homeomorphism with derivative $E \cdot D_7$ that carries $S_7$ to $E \cdot \omega_7$.

As discussed above, $1 \cdot \eta_s$ is forward asymptotic to the sum of $\eta_s$ over all automorphisms of $K$. We compute this below:

[39]:
```
k = k_def(7)
K = K_def(k)
sum_over_automorphisms(K, eta_s)
```

[39]: (0, 0, -1, 1, 1, 0, -1)

This list gives $[\Psi_c](e_i)$ for $i = 0, \ldots, 6$.
